# Supplementary material for: Self-dual, self-Petrie-dual and M\"obius regular maps on linear fractional groups
Source: arXiv:1807.11307 ancillary file (2018-07-30)
Supplement: Supplementary file 1 [file SD_SPD_MR_Maps_on_LFG_Ancillary.pdf]

**ANCILLARY FILE FOR:  
SELF-DUAL, SELF-PETRIE-DUAL AND MÖBIUS REGULAR  
MAPS ON LINEAR FRACTIONAL GROUPS.**

Grahame Erskine

Open University, Milton Keynes, U.K.  
grahame.erskine@open.ac.uk

Katarína Hriňáková

Slovak University of Technology, Bratislava, Slovakia  
hrinakova@math.sk

and

Olivia Jeans

Open University, Milton Keynes, U.K.  
olivia.jeans@open.ac.uk

1. EXTENDED TABLES OF RESULTS

In the following tables, produced using the computer package GAP [1], we list for given  $q \leq 81$ , all the  $PSL(2, q)$  maps which have one or more of the properties we have addressed in the paper, the ticks indicating when the map has each property. The elements  $\xi_\kappa$ ,  $\xi_\lambda$ ,  $\omega_\kappa$  and  $\omega_\lambda$  are expressed as powers of a primitive element  $\xi$  in the field  $GF(q^2)$ . For a given  $k, l$ , only one map is shown in each equivalence class under the action of the automorphism group.

For interest we also include an enumeration in Table 2 which shows how many  $PSL(2, q)$  maps there are with each of these combinations of properties for  $q \leq 81$ .

TABLES

| $q$ | $k$ | $l$ | $\log_\xi \xi_\kappa$ | $\log_\xi \xi_\lambda$ | $\log_\xi \omega_\kappa$ | $\log_\xi \omega_\lambda$ | SD | SPD | MR |
|-----|-----|-----|-----------------------|------------------------|--------------------------|---------------------------|----|-----|----|
| 5   | 5   | 5   |                       |                        |                          |                           | ✓  |     |    |
| 7   | 7   | 7   |                       |                        |                          |                           | ✓  |     |    |
| 9   | 5   | 5   | 8                     | 8                      | 30                       | 30                        | ✓  |     |    |
| 11  | 5   | 5   | 12                    | 12                     | 36                       | 36                        | ✓  |     |    |
| 11  | 5   | 5   | 36                    | 36                     | 24                       | 24                        | ✓  | ✓   |    |
| 11  | 5   | 6   | 12                    | 10                     | 36                       | 108                       |    |     | ✓  |
| 11  | 6   | 6   | 10                    | 10                     | 108                      | 108                       | ✓  |     |    |
| 11  | 11  | 11  |                       |                        |                          |                           | ✓  |     |    |
| 13  | 6   | 6   | 14                    | 14                     | 112                      | 112                       | ✓  |     |    |
| 13  | 7   | 7   | 12                    | 12                     | 126                      | 126                       | ✓  |     |    |
| 13  | 7   | 7   | 12                    | 60                     | 126                      | 56                        |    |     | ✓  |

| $q$ | $k$ | $l$ | $\log_{\xi} \xi_{\kappa}$ | $\log_{\xi} \xi_{\lambda}$ | $\log_{\xi} \omega_{\kappa}$ | $\log_{\xi} \omega_{\lambda}$ | SD | SPD | MR |
|-----|-----|-----|---------------------------|----------------------------|------------------------------|-------------------------------|----|-----|----|
| 13  | 7   | 7   | 36                        | 36                         | 70                           | 70                            | ✓  | ✓   |    |
| 13  | 7   | 7   | 60                        | 60                         | 56                           | 56                            | ✓  |     |    |
| 13  | 7   | 13  | 60                        |                            | 56                           |                               |    | ✓   |    |
| 13  | 13  | 13  |                           |                            |                              |                               | ✓  |     |    |
| 17  | 8   | 8   | 18                        | 18                         | 36                           | 36                            | ✓  |     |    |
| 17  | 8   | 8   | 54                        | 54                         | 90                           | 90                            | ✓  |     |    |
| 17  | 8   | 9   | 54                        | 80                         | 90                           | 54                            |    | ✓   | ✓  |
| 17  | 8   | 17  | 18                        |                            | 36                           |                               |    | ✓   | ✓  |
| 17  | 9   | 9   | 16                        | 16                         | 216                          | 216                           | ✓  |     |    |
| 17  | 9   | 9   | 80                        | 80                         | 54                           | 54                            | ✓  |     |    |
| 17  | 9   | 9   | 112                       | 112                        | 18                           | 18                            | ✓  |     |    |
| 17  | 17  | 17  |                           |                            |                              |                               | ✓  |     |    |
| 19  | 3   | 9   | 60                        | 20                         | 0                            | 300                           |    | ✓   |    |
| 19  | 5   | 5   | 36                        | 36                         | 320                          | 320                           | ✓  |     |    |
| 19  | 5   | 5   | 108                       | 108                        | 220                          | 220                           | ✓  |     |    |
| 19  | 9   | 5   | 20                        | 36                         | 300                          | 320                           |    | ✓   |    |
| 19  | 9   | 9   | 20                        | 20                         | 300                          | 300                           | ✓  |     |    |
| 19  | 9   | 9   | 100                       | 100                        | 80                           | 80                            | ✓  |     |    |
| 19  | 9   | 9   | 140                       | 100                        | 340                          | 80                            |    | ✓   |    |
| 19  | 9   | 9   | 140                       | 140                        | 340                          | 340                           | ✓  |     |    |
| 19  | 9   | 10  | 100                       | 18                         | 80                           | 60                            |    | ✓   |    |
| 19  | 10  | 10  | 18                        | 18                         | 60                           | 60                            | ✓  |     |    |
| 19  | 10  | 10  | 54                        | 54                         | 100                          | 100                           | ✓  |     |    |
| 19  | 19  | 19  |                           |                            |                              |                               | ✓  |     |    |
| 23  | 3   | 11  | 88                        | 72                         | 0                            | 168                           |    | ✓   |    |
| 23  | 6   | 6   | 44                        | 44                         | 192                          | 192                           | ✓  |     |    |
| 23  | 6   | 11  | 44                        | 216                        | 192                          | 240                           |    | ✓   | ✓  |
| 23  | 11  | 11  | 24                        | 24                         | 360                          | 360                           | ✓  |     |    |
| 23  | 11  | 11  | 72                        | 72                         | 168                          | 168                           | ✓  |     |    |
| 23  | 11  | 11  | 120                       | 120                        | 480                          | 480                           | ✓  |     |    |
| 23  | 11  | 11  | 168                       | 168                        | 336                          | 336                           | ✓  |     |    |
| 23  | 11  | 11  | 216                       | 216                        | 240                          | 240                           | ✓  |     |    |
| 23  | 12  | 11  | 22                        | 24                         | 144                          | 360                           |    | ✓   | ✓  |
| 23  | 12  | 12  | 22                        | 22                         | 144                          | 144                           | ✓  |     |    |
| 23  | 12  | 12  | 110                       | 110                        | 384                          | 384                           | ✓  | ✓   | ✓  |
| 23  | 23  | 23  |                           |                            |                              |                               | ✓  |     |    |
| 25  | 3   | 13  | 104                       | 72                         | 0                            | 494                           |    | ✓   |    |
| 25  | 4   | 13  | 78                        | 168                        | 390                          | 26                            |    | ✓   |    |
| 25  | 6   | 13  | 52                        | 24                         | 546                          | 260                           |    | ✓   |    |
| 25  | 12  | 12  | 26                        | 26                         | 416                          | 416                           | ✓  |     |    |
| 25  | 12  | 13  | 26                        | 216                        | 416                          | 130                           |    | ✓   | ✓  |
| 25  | 13  | 13  | 24                        | 24                         | 260                          | 260                           | ✓  |     |    |
| 25  | 13  | 13  | 24                        | 120                        | 260                          | 52                            | ✓  |     |    |
| 25  | 13  | 13  | 72                        | 72                         | 494                          | 494                           | ✓  |     |    |
| 25  | 13  | 13  | 72                        | 264                        | 494                          | 598                           | ✓  |     |    |
| 25  | 13  | 13  | 168                       | 168                        | 26                           | 26                            | ✓  |     |    |
| 25  | 13  | 13  | 168                       | 216                        | 26                           | 130                           | ✓  |     |    |

| $q$ | $k$ | $l$ | $\log_{\xi} \xi_{\kappa}$ | $\log_{\xi} \xi_{\lambda}$ | $\log_{\xi} \omega_{\kappa}$ | $\log_{\xi} \omega_{\lambda}$ | SD | SPD | MR |
|-----|-----|-----|---------------------------|----------------------------|------------------------------|-------------------------------|----|-----|----|
| 27  | 7   | 7   | 52                        | 52                         | 420                          | 420                           | ✓  |     |    |
| 27  | 13  | 7   | 140                       | 156                        | 28                           | 532                           |    | ✓   |    |
| 27  | 13  | 13  | 28                        | 28                         | 560                          | 560                           | ✓  |     |    |
| 27  | 13  | 13  | 28                        | 252                        | 560                          | 672                           |    | ✓   |    |
| 27  | 13  | 13  | 140                       | 140                        | 28                           | 28                            | ✓  |     |    |
| 27  | 14  | 14  | 26                        | 26                         | 476                          | 476                           | ✓  |     |    |
| 29  | 3   | 15  | 140                       | 28                         | 0                            | 480                           |    | ✓   |    |
| 29  | 5   | 5   | 84                        | 84                         | 180                          | 180                           | ✓  |     |    |
| 29  | 5   | 5   | 252                       | 252                        | 240                          | 240                           | ✓  |     |    |
| 29  | 5   | 14  | 84                        | 90                         | 180                          | 270                           |    | ✓   |    |
| 29  | 5   | 29  | 252                       |                            | 240                          |                               |    | ✓   |    |
| 29  | 7   | 7   | 60                        | 60                         | 570                          | 570                           | ✓  |     |    |
| 29  | 7   | 7   | 180                       | 180                        | 750                          | 750                           | ✓  |     |    |
| 29  | 7   | 7   | 300                       | 300                        | 780                          | 780                           | ✓  |     |    |
| 29  | 14  | 14  | 30                        | 30                         | 630                          | 630                           | ✓  |     |    |
| 29  | 14  | 14  | 90                        | 90                         | 270                          | 270                           | ✓  |     |    |
| 29  | 14  | 14  | 150                       | 150                        | 540                          | 540                           | ✓  |     |    |
| 29  | 15  | 7   | 308                       | 180                        | 300                          | 750                           |    | ✓   |    |
| 29  | 15  | 7   | 364                       | 300                        | 810                          | 780                           |    | ✓   |    |
| 29  | 15  | 14  | 196                       | 30                         | 90                           | 630                           |    | ✓   |    |
| 29  | 15  | 15  | 28                        | 28                         | 480                          | 480                           | ✓  |     |    |
| 29  | 15  | 15  | 28                        | 308                        | 480                          | 300                           |    | ✓   |    |
| 29  | 15  | 15  | 196                       | 196                        | 90                           | 90                            | ✓  |     |    |
| 29  | 15  | 15  | 308                       | 308                        | 300                          | 300                           | ✓  |     |    |
| 29  | 15  | 15  | 364                       | 364                        | 810                          | 810                           | ✓  |     |    |
| 29  | 29  | 29  |                           |                            |                              |                               | ✓  |     |    |
| 31  | 5   | 5   | 96                        | 96                         | 128                          | 128                           | ✓  |     |    |
| 31  | 5   | 5   | 288                       | 288                        | 352                          | 352                           | ✓  |     |    |
| 31  | 8   | 8   | 60                        | 60                         | 160                          | 160                           | ✓  |     |    |
| 31  | 8   | 8   | 180                       | 180                        | 704                          | 704                           | ✓  |     |    |
| 31  | 8   | 15  | 60                        | 352                        | 160                          | 320                           |    | ✓   | ✓  |
| 31  | 8   | 16  | 180                       | 30                         | 704                          | 256                           |    | ✓   | ✓  |
| 31  | 15  | 15  | 32                        | 32                         | 416                          | 416                           | ✓  |     |    |
| 31  | 15  | 15  | 224                       | 224                        | 512                          | 512                           | ✓  |     |    |
| 31  | 15  | 15  | 352                       | 352                        | 320                          | 320                           | ✓  |     |    |
| 31  | 15  | 15  | 416                       | 416                        | 672                          | 672                           | ✓  |     |    |
| 31  | 16  | 5   | 210                       | 288                        | 448                          | 352                           |    | ✓   | ✓  |
| 31  | 16  | 8   | 90                        | 60                         | 576                          | 160                           |    | ✓   | ✓  |
| 31  | 16  | 15  | 150                       | 416                        | 544                          | 672                           |    | ✓   | ✓  |
| 31  | 16  | 16  | 30                        | 30                         | 256                          | 256                           | ✓  |     |    |
| 31  | 16  | 16  | 30                        | 150                        | 256                          | 544                           |    | ✓   | ✓  |
| 31  | 16  | 16  | 90                        | 90                         | 576                          | 576                           | ✓  |     |    |
| 31  | 16  | 16  | 150                       | 150                        | 544                          | 544                           | ✓  |     |    |
| 31  | 16  | 16  | 210                       | 210                        | 448                          | 448                           | ✓  |     |    |
| 31  | 31  | 31  |                           |                            |                              |                               | ✓  |     |    |
| 37  | 6   | 6   | 114                       | 114                        | 1178                         | 1178                          | ✓  |     |    |
| 37  | 9   | 9   | 76                        | 76                         | 190                          | 190                           | ✓  |     |    |

| $q$ | $k$ | $l$ | $\log_{\xi} \xi_{\kappa}$ | $\log_{\xi} \xi_{\lambda}$ | $\log_{\xi} \omega_{\kappa}$ | $\log_{\xi} \omega_{\lambda}$ | SD | SPD | MR |
|-----|-----|-----|---------------------------|----------------------------|------------------------------|-------------------------------|----|-----|----|
| 37  | 9   | 9   | 380                       | 380                        | 1292                         | 1292                          | ✓  |     |    |
| 37  | 9   | 9   | 532                       | 532                        | 1254                         | 1254                          | ✓  |     |    |
| 37  | 18  | 18  | 38                        | 38                         | 836                          | 836                           | ✓  |     |    |
| 37  | 18  | 18  | 190                       | 190                        | 266                          | 266                           | ✓  |     |    |
| 37  | 18  | 18  | 266                       | 266                        | 76                           | 76                            | ✓  |     |    |
| 37  | 19  | 9   | 180                       | 380                        | 798                          | 1292                          |    | ✓   |    |
| 37  | 19  | 9   | 468                       | 76                         | 646                          | 190                           |    | ✓   |    |
| 37  | 19  | 18  | 252                       | 38                         | 1140                         | 836                           |    | ✓   |    |
| 37  | 19  | 18  | 612                       | 266                        | 988                          | 76                            |    | ✓   |    |
| 37  | 19  | 19  | 36                        | 36                         | 1026                         | 1026                          | ✓  |     |    |
| 37  | 19  | 19  | 36                        | 108                        | 1026                         | 418                           |    | ✓   |    |
| 37  | 19  | 19  | 108                       | 108                        | 418                          | 418                           | ✓  |     |    |
| 37  | 19  | 19  | 108                       | 252                        | 418                          | 1140                          |    | ✓   |    |
| 37  | 19  | 19  | 180                       | 180                        | 798                          | 798                           | ✓  |     |    |
| 37  | 19  | 19  | 252                       | 252                        | 1140                         | 1140                          | ✓  |     |    |
| 37  | 19  | 19  | 324                       | 324                        | 1064                         | 1064                          | ✓  |     |    |
| 37  | 19  | 19  | 396                       | 396                        | 228                          | 228                           | ✓  | ✓   |    |
| 37  | 19  | 19  | 468                       | 468                        | 646                          | 646                           | ✓  |     |    |
| 37  | 19  | 19  | 540                       | 324                        | 532                          | 1064                          |    | ✓   |    |
| 37  | 19  | 19  | 540                       | 540                        | 532                          | 532                           | ✓  |     |    |
| 37  | 19  | 19  | 612                       | 612                        | 988                          | 988                           | ✓  |     |    |
| 37  | 19  | 37  | 324                       |                            | 1064                         |                               |    | ✓   |    |
| 37  | 37  | 37  |                           |                            |                              |                               | ✓  |     |    |
| 41  | 5   | 5   | 168                       | 168                        | 1638                         | 1638                          | ✓  |     |    |
| 41  | 5   | 5   | 504                       | 504                        | 882                          | 882                           | ✓  |     |    |
| 41  | 5   | 7   | 168                       | 600                        | 1638                         | 126                           |    | ✓   |    |
| 41  | 5   | 20  | 504                       | 294                        | 882                          | 924                           |    | ✓   |    |
| 41  | 7   | 7   | 120                       | 120                        | 210                          | 210                           | ✓  |     |    |
| 41  | 7   | 7   | 360                       | 360                        | 504                          | 504                           | ✓  |     |    |
| 41  | 7   | 7   | 600                       | 600                        | 126                          | 126                           | ✓  |     |    |
| 41  | 10  | 10  | 84                        | 84                         | 630                          | 630                           | ✓  |     |    |
| 41  | 10  | 10  | 252                       | 252                        | 672                          | 672                           | ✓  |     |    |
| 41  | 10  | 21  | 84                        | 520                        | 630                          | 336                           |    | ✓   | ✓  |
| 41  | 10  | 41  | 252                       |                            | 672                          |                               |    | ✓   | ✓  |
| 41  | 20  | 20  | 42                        | 42                         | 1302                         | 1302                          | ✓  |     |    |
| 41  | 20  | 20  | 42                        | 126                        | 1302                         | 714                           |    | ✓   | ✓  |
| 41  | 20  | 20  | 126                       | 126                        | 714                          | 714                           | ✓  |     |    |
| 41  | 20  | 20  | 294                       | 294                        | 924                          | 924                           | ✓  |     |    |
| 41  | 20  | 20  | 378                       | 378                        | 420                          | 420                           | ✓  |     |    |
| 41  | 20  | 21  | 126                       | 680                        | 714                          | 1218                          |    | ✓   | ✓  |
| 41  | 20  | 21  | 294                       | 200                        | 924                          | 168                           |    | ✓   | ✓  |
| 41  | 20  | 21  | 378                       | 440                        | 420                          | 756                           |    | ✓   | ✓  |
| 41  | 21  | 21  | 40                        | 40                         | 1428                         | 1428                          | ✓  |     |    |
| 41  | 21  | 21  | 200                       | 200                        | 168                          | 168                           | ✓  |     |    |
| 41  | 21  | 21  | 440                       | 440                        | 756                          | 756                           | ✓  |     |    |
| 41  | 21  | 21  | 520                       | 520                        | 336                          | 336                           | ✓  |     |    |
| 41  | 21  | 21  | 680                       | 680                        | 1218                         | 1218                          | ✓  |     |    |

| $q$ | $k$ | $l$ | $\log_{\xi} \xi_{\kappa}$ | $\log_{\xi} \xi_{\lambda}$ | $\log_{\xi} \omega_{\kappa}$ | $\log_{\xi} \omega_{\lambda}$ | SD | SPD | MR |
|-----|-----|-----|---------------------------|----------------------------|------------------------------|-------------------------------|----|-----|----|
| 41  | 21  | 21  | 760                       | 760                        | 1134                         | 1134                          | ✓  |     |    |
| 41  | 41  | 41  |                           |                            |                              |                               | ✓  |     |    |
| 43  | 3   | 22  | 308                       | 294                        | 0                            | 1276                          |    | ✓   |    |
| 43  | 7   | 7   | 132                       | 132                        | 792                          | 792                           | ✓  |     |    |
| 43  | 7   | 7   | 396                       | 396                        | 220                          | 220                           | ✓  |     |    |
| 43  | 7   | 7   | 660                       | 660                        | 1760                         | 1760                          | ✓  |     |    |
| 43  | 7   | 21  | 132                       | 484                        | 792                          | 1628                          |    | ✓   |    |
| 43  | 7   | 21  | 396                       | 572                        | 220                          | 484                           |    | ✓   |    |
| 43  | 7   | 21  | 660                       | 748                        | 1760                         | 1496                          |    | ✓   |    |
| 43  | 11  | 11  | 84                        | 84                         | 1452                         | 1452                          | ✓  |     |    |
| 43  | 11  | 11  | 252                       | 252                        | 1012                         | 1012                          | ✓  |     |    |
| 43  | 11  | 11  | 420                       | 420                        | 1540                         | 1540                          | ✓  |     |    |
| 43  | 11  | 11  | 588                       | 588                        | 1584                         | 1584                          | ✓  |     |    |
| 43  | 11  | 11  | 756                       | 756                        | 1804                         | 1804                          | ✓  |     |    |
| 43  | 21  | 7   | 484                       | 660                        | 1628                         | 1760                          |    | ✓   |    |
| 43  | 21  | 11  | 44                        | 420                        | 396                          | 1540                          |    | ✓   |    |
| 43  | 21  | 11  | 220                       | 588                        | 1100                         | 1584                          |    | ✓   |    |
| 43  | 21  | 11  | 748                       | 84                         | 1496                         | 1452                          |    | ✓   |    |
| 43  | 21  | 11  | 836                       | 252                        | 440                          | 1012                          |    | ✓   |    |
| 43  | 21  | 21  | 44                        | 44                         | 396                          | 396                           | ✓  |     |    |
| 43  | 21  | 21  | 220                       | 220                        | 1100                         | 1100                          | ✓  |     |    |
| 43  | 21  | 21  | 484                       | 484                        | 1628                         | 1628                          | ✓  |     |    |
| 43  | 21  | 21  | 572                       | 220                        | 484                          | 1100                          |    | ✓   |    |
| 43  | 21  | 21  | 572                       | 572                        | 484                          | 484                           | ✓  |     |    |
| 43  | 21  | 21  | 748                       | 748                        | 1496                         | 1496                          | ✓  |     |    |
| 43  | 21  | 21  | 836                       | 836                        | 440                          | 440                           | ✓  |     |    |
| 43  | 22  | 22  | 42                        | 42                         | 132                          | 132                           | ✓  |     |    |
| 43  | 22  | 22  | 126                       | 126                        | 308                          | 308                           | ✓  |     |    |
| 43  | 22  | 22  | 210                       | 210                        | 968                          | 968                           | ✓  |     |    |
| 43  | 22  | 22  | 294                       | 294                        | 1276                         | 1276                          | ✓  |     |    |
| 43  | 22  | 22  | 378                       | 378                        | 1672                         | 1672                          | ✓  |     |    |
| 43  | 43  | 43  |                           |                            |                              |                               | ✓  |     |    |
| 47  | 3   | 23  | 368                       | 528                        | 0                            | 1152                          |    | ✓   |    |
| 47  | 6   | 6   | 184                       | 184                        | 480                          | 480                           | ✓  |     |    |
| 47  | 6   | 24  | 184                       | 46                         | 480                          | 672                           |    | ✓   | ✓  |
| 47  | 8   | 8   | 138                       | 138                        | 960                          | 960                           | ✓  |     |    |
| 47  | 8   | 8   | 414                       | 414                        | 576                          | 576                           | ✓  |     |    |
| 47  | 8   | 23  | 138                       | 624                        | 960                          | 144                           |    | ✓   | ✓  |
| 47  | 8   | 23  | 414                       | 432                        | 576                          | 528                           |    | ✓   | ✓  |
| 47  | 12  | 8   | 92                        | 414                        | 1200                         | 576                           |    | ✓   | ✓  |
| 47  | 12  | 12  | 92                        | 92                         | 1200                         | 1200                          | ✓  |     |    |
| 47  | 12  | 12  | 460                       | 460                        | 1008                         | 1008                          | ✓  |     |    |
| 47  | 12  | 23  | 460                       | 816                        | 1008                         | 768                           |    | ✓   | ✓  |
| 47  | 23  | 23  | 48                        | 48                         | 1344                         | 1344                          | ✓  |     |    |
| 47  | 23  | 23  | 144                       | 144                        | 1056                         | 1056                          | ✓  |     |    |
| 47  | 23  | 23  | 240                       | 240                        | 288                          | 288                           | ✓  |     |    |
| 47  | 23  | 23  | 336                       | 336                        | 720                          | 720                           | ✓  |     |    |

| $q$ | $k$ | $l$ | $\log_{\xi} \xi_{\kappa}$ | $\log_{\xi} \xi_{\lambda}$ | $\log_{\xi} \omega_{\kappa}$ | $\log_{\xi} \omega_{\lambda}$ | SD | SPD | MR |
|-----|-----|-----|---------------------------|----------------------------|------------------------------|-------------------------------|----|-----|----|
| 47  | 23  | 23  | 432                       | 432                        | 528                          | 528                           | ✓  |     |    |
| 47  | 23  | 23  | 528                       | 528                        | 1152                         | 1152                          | ✓  |     |    |
| 47  | 23  | 23  | 624                       | 624                        | 144                          | 144                           | ✓  |     |    |
| 47  | 23  | 23  | 720                       | 720                        | 1296                         | 1296                          | ✓  |     |    |
| 47  | 23  | 23  | 816                       | 816                        | 768                          | 768                           | ✓  |     |    |
| 47  | 23  | 23  | 912                       | 912                        | 624                          | 624                           | ✓  |     |    |
| 47  | 23  | 23  | 1008                      | 1008                       | 2016                         | 2016                          | ✓  |     |    |
| 47  | 24  | 12  | 46                        | 460                        | 672                          | 1008                          |    | ✓   | ✓  |
| 47  | 24  | 23  | 322                       | 144                        | 1920                         | 1056                          |    | ✓   | ✓  |
| 47  | 24  | 23  | 506                       | 48                         | 336                          | 1344                          |    | ✓   | ✓  |
| 47  | 24  | 24  | 46                        | 46                         | 672                          | 672                           | ✓  |     |    |
| 47  | 24  | 24  | 230                       | 230                        | 1488                         | 1488                          | ✓  | ✓   | ✓  |
| 47  | 24  | 24  | 322                       | 322                        | 1920                         | 1920                          | ✓  |     |    |
| 47  | 24  | 24  | 506                       | 506                        | 336                          | 336                           | ✓  |     |    |
| 47  | 47  | 47  |                           |                            |                              |                               | ✓  |     |    |
| 49  | 4   | 25  | 300                       | 144                        | 400                          | 1250                          |    | ✓   |    |
| 49  | 5   | 5   | 240                       | 240                        | 1350                         | 1350                          | ✓  |     |    |
| 49  | 6   | 24  | 200                       | 250                        | 1400                         | 2050                          |    | ✓   |    |
| 49  | 7   | 24  |                           | 50                         |                              | 500                           |    | ✓   |    |
| 49  | 7   | 25  |                           | 432                        |                              | 1500                          |    | ✓   |    |
| 49  | 7   | 25  |                           | 816                        |                              | 100                           |    | ✓   |    |
| 49  | 8   | 25  | 150                       | 48                         | 2200                         | 1450                          |    | ✓   |    |
| 49  | 8   | 25  | 450                       | 528                        | 600                          | 950                           |    | ✓   |    |
| 49  | 12  | 12  | 100                       | 100                        | 750                          | 750                           | ✓  |     |    |
| 49  | 12  | 25  | 100                       | 144                        | 750                          | 1250                          |    | ✓   | ✓  |
| 49  | 24  | 12  | 50                        | 100                        | 500                          | 750                           |    | ✓   | ✓  |
| 49  | 24  | 24  | 50                        | 50                         | 500                          | 500                           | ✓  |     |    |
| 49  | 24  | 24  | 50                        | 350                        | 500                          | 1100                          | ✓  |     |    |
| 49  | 24  | 24  | 250                       | 250                        | 2050                         | 2050                          | ✓  |     |    |
| 49  | 24  | 24  | 250                       | 550                        | 2050                         | 1150                          | ✓  |     |    |
| 49  | 24  | 25  | 250                       | 912                        | 2050                         | 700                           |    | ✓   | ✓  |
| 49  | 25  | 25  | 48                        | 48                         | 1450                         | 1450                          | ✓  |     |    |
| 49  | 25  | 25  | 48                        | 336                        | 1450                         | 550                           | ✓  |     |    |
| 49  | 25  | 25  | 144                       | 144                        | 1250                         | 1250                          | ✓  |     |    |
| 49  | 25  | 25  | 144                       | 1008                       | 1250                         | 1550                          | ✓  |     |    |
| 49  | 25  | 25  | 432                       | 432                        | 1500                         | 1500                          | ✓  |     |    |
| 49  | 25  | 25  | 432                       | 624                        | 1500                         | 900                           | ✓  |     |    |
| 49  | 25  | 25  | 528                       | 528                        | 950                          | 950                           | ✓  |     |    |
| 49  | 25  | 25  | 528                       | 1104                       | 950                          | 1850                          | ✓  |     |    |
| 49  | 25  | 25  | 816                       | 816                        | 100                          | 100                           | ✓  |     |    |
| 49  | 25  | 25  | 816                       | 912                        | 100                          | 700                           | ✓  |     |    |
| 53  | 3   | 13  | 468                       | 108                        | 0                            | 432                           |    | ✓   |    |
| 53  | 9   | 9   | 156                       | 156                        | 2214                         | 2214                          | ✓  |     |    |
| 53  | 9   | 9   | 780                       | 780                        | 1512                         | 1512                          | ✓  |     |    |
| 53  | 9   | 9   | 1092                      | 1092                       | 1890                         | 1890                          | ✓  |     |    |
| 53  | 9   | 13  | 156                       | 324                        | 2214                         | 2700                          |    | ✓   |    |
| 53  | 9   | 26  | 780                       | 378                        | 1512                         | 2592                          |    | ✓   |    |

| $q$ | $k$ | $l$ | $\log_{\xi} \xi_{\kappa}$ | $\log_{\xi} \xi_{\lambda}$ | $\log_{\xi} \omega_{\kappa}$ | $\log_{\xi} \omega_{\lambda}$ | SD | SPD | MR |
|-----|-----|-----|---------------------------|----------------------------|------------------------------|-------------------------------|----|-----|----|
| 53  | 9   | 27  | 1092                      | 884                        | 1890                         | 702                           |    | ✓   |    |
| 53  | 13  | 13  | 108                       | 108                        | 432                          | 432                           | ✓  |     |    |
| 53  | 13  | 13  | 324                       | 324                        | 2700                         | 2700                          | ✓  |     |    |
| 53  | 13  | 13  | 540                       | 540                        | 1728                         | 1728                          | ✓  |     |    |
| 53  | 13  | 13  | 756                       | 756                        | 1566                         | 1566                          | ✓  |     |    |
| 53  | 13  | 13  | 972                       | 972                        | 648                          | 648                           | ✓  |     |    |
| 53  | 13  | 13  | 1188                      | 1188                       | 2754                         | 2754                          | ✓  |     |    |
| 53  | 26  | 26  | 54                        | 54                         | 2484                         | 2484                          | ✓  |     |    |
| 53  | 26  | 26  | 162                       | 162                        | 864                          | 864                           | ✓  |     |    |
| 53  | 26  | 26  | 270                       | 270                        | 1620                         | 1620                          | ✓  |     |    |
| 53  | 26  | 26  | 378                       | 378                        | 2592                         | 2592                          | ✓  |     |    |
| 53  | 26  | 26  | 486                       | 486                        | 270                          | 270                           | ✓  |     |    |
| 53  | 26  | 26  | 594                       | 594                        | 2646                         | 2646                          | ✓  |     |    |
| 53  | 27  | 9   | 52                        | 156                        | 972                          | 2214                          |    | ✓   |    |
| 53  | 27  | 9   | 260                       | 780                        | 1134                         | 1512                          |    | ✓   |    |
| 53  | 27  | 26  | 884                       | 594                        | 702                          | 2646                          |    | ✓   |    |
| 53  | 27  | 27  | 52                        | 52                         | 972                          | 972                           | ✓  |     |    |
| 53  | 27  | 27  | 260                       | 260                        | 1134                         | 1134                          | ✓  |     |    |
| 53  | 27  | 27  | 364                       | 364                        | 918                          | 918                           | ✓  |     |    |
| 53  | 27  | 27  | 364                       | 988                        | 918                          | 540                           |    | ✓   |    |
| 53  | 27  | 27  | 572                       | 260                        | 1782                         | 1134                          |    | ✓   |    |
| 53  | 27  | 27  | 572                       | 572                        | 1782                         | 1782                          | ✓  |     |    |
| 53  | 27  | 27  | 676                       | 676                        | 2160                         | 2160                          | ✓  |     |    |
| 53  | 27  | 27  | 884                       | 884                        | 702                          | 702                           | ✓  |     |    |
| 53  | 27  | 27  | 988                       | 988                        | 540                          | 540                           | ✓  |     |    |
| 53  | 27  | 27  | 988                       | 1300                       | 540                          | 1998                          |    | ✓   |    |
| 53  | 27  | 27  | 1196                      | 52                         | 1026                         | 972                           |    | ✓   |    |
| 53  | 27  | 27  | 1196                      | 1196                       | 1026                         | 1026                          | ✓  |     |    |
| 53  | 27  | 27  | 1300                      | 572                        | 1998                         | 1782                          |    | ✓   |    |
| 53  | 27  | 27  | 1300                      | 1300                       | 1998                         | 1998                          | ✓  |     |    |
| 53  | 27  | 53  | 676                       |                            | 2160                         |                               |    | ✓   |    |
| 53  | 53  | 53  |                           |                            |                              |                               | ✓  |     |    |
| 59  | 5   | 5   | 348                       | 348                        | 2760                         | 2760                          | ✓  |     |    |
| 59  | 5   | 5   | 1044                      | 1044                       | 2460                         | 2460                          | ✓  |     |    |
| 59  | 6   | 6   | 290                       | 290                        | 1500                         | 1500                          | ✓  |     |    |
| 59  | 10  | 10  | 174                       | 174                        | 2340                         | 2340                          | ✓  |     |    |
| 59  | 10  | 10  | 522                       | 522                        | 3060                         | 3060                          | ✓  |     |    |
| 59  | 15  | 15  | 116                       | 116                        | 3360                         | 3360                          | ✓  |     |    |
| 59  | 15  | 15  | 812                       | 812                        | 480                          | 480                           | ✓  |     |    |
| 59  | 15  | 15  | 1276                      | 1276                       | 420                          | 420                           | ✓  |     |    |
| 59  | 15  | 15  | 1508                      | 1508                       | 2700                         | 2700                          | ✓  |     |    |
| 59  | 29  | 5   | 300                       | 348                        | 1260                         | 2760                          |    | ✓   |    |
| 59  | 29  | 6   | 1260                      | 290                        | 2640                         | 1500                          |    | ✓   |    |
| 59  | 29  | 10  | 1620                      | 174                        | 540                          | 2340                          |    | ✓   |    |
| 59  | 29  | 15  | 420                       | 1508                       | 240                          | 2700                          |    | ✓   |    |
| 59  | 29  | 15  | 540                       | 116                        | 3120                         | 3360                          |    | ✓   |    |
| 59  | 29  | 29  | 60                        | 60                         | 300                          | 300                           | ✓  | ✓   |    |

| $q$ | $k$ | $l$ | $\log_{\xi} \xi_{\kappa}$ | $\log_{\xi} \xi_{\lambda}$ | $\log_{\xi} \omega_{\kappa}$ | $\log_{\xi} \omega_{\lambda}$ | SD | SPD | MR |
|-----|-----|-----|---------------------------|----------------------------|------------------------------|-------------------------------|----|-----|----|
| 59  | 29  | 29  | 180                       | 180                        | 2880                         | 2880                          | ✓  |     |    |
| 59  | 29  | 29  | 300                       | 300                        | 1260                         | 1260                          | ✓  |     |    |
| 59  | 29  | 29  | 420                       | 420                        | 240                          | 240                           | ✓  |     |    |
| 59  | 29  | 29  | 540                       | 540                        | 3120                         | 3120                          | ✓  |     |    |
| 59  | 29  | 29  | 660                       | 300                        | 1440                         | 1260                          |    | ✓   |    |
| 59  | 29  | 29  | 660                       | 660                        | 1440                         | 1440                          | ✓  |     |    |
| 59  | 29  | 29  | 780                       | 780                        | 120                          | 120                           | ✓  |     |    |
| 59  | 29  | 29  | 780                       | 1380                       | 120                          | 660                           |    | ✓   |    |
| 59  | 29  | 29  | 900                       | 900                        | 840                          | 840                           | ✓  |     |    |
| 59  | 29  | 29  | 1020                      | 900                        | 180                          | 840                           |    | ✓   |    |
| 59  | 29  | 29  | 1020                      | 1020                       | 180                          | 180                           | ✓  |     |    |
| 59  | 29  | 29  | 1140                      | 1140                       | 2820                         | 2820                          | ✓  |     |    |
| 59  | 29  | 29  | 1140                      | 1620                       | 2820                         | 540                           |    | ✓   |    |
| 59  | 29  | 29  | 1260                      | 1260                       | 2640                         | 2640                          | ✓  |     |    |
| 59  | 29  | 29  | 1380                      | 1020                       | 660                          | 180                           |    | ✓   |    |
| 59  | 29  | 29  | 1380                      | 1380                       | 660                          | 660                           | ✓  |     |    |
| 59  | 29  | 29  | 1500                      | 180                        | 2100                         | 2880                          |    | ✓   |    |
| 59  | 29  | 29  | 1500                      | 1500                       | 2100                         | 2100                          | ✓  |     |    |
| 59  | 29  | 29  | 1620                      | 1620                       | 540                          | 540                           | ✓  |     |    |
| 59  | 29  | 30  | 180                       | 406                        | 2880                         | 2520                          |    | ✓   |    |
| 59  | 29  | 30  | 900                       | 58                         | 840                          | 1200                          |    | ✓   |    |
| 59  | 30  | 30  | 58                        | 58                         | 1200                         | 1200                          | ✓  |     |    |
| 59  | 30  | 30  | 406                       | 406                        | 2520                         | 2520                          | ✓  |     |    |
| 59  | 30  | 30  | 638                       | 638                        | 1560                         | 1560                          | ✓  |     |    |
| 59  | 30  | 30  | 754                       | 754                        | 1680                         | 1680                          | ✓  |     |    |
| 59  | 59  | 59  |                           |                            |                              |                               | ✓  |     |    |
| 61  | 5   | 5   | 372                       | 372                        | 1054                         | 1054                          | ✓  |     |    |
| 61  | 5   | 5   | 1116                      | 1116                       | 806                          | 806                           | ✓  |     |    |
| 61  | 6   | 6   | 310                       | 310                        | 2046                         | 2046                          | ✓  |     |    |
| 61  | 10  | 10  | 186                       | 186                        | 3658                         | 3658                          | ✓  |     |    |
| 61  | 10  | 10  | 558                       | 558                        | 2604                         | 2604                          | ✓  |     |    |
| 61  | 15  | 15  | 124                       | 124                        | 2790                         | 2790                          | ✓  |     |    |
| 61  | 15  | 15  | 868                       | 868                        | 3100                         | 3100                          | ✓  |     |    |
| 61  | 15  | 15  | 1364                      | 1364                       | 1178                         | 1178                          | ✓  |     |    |
| 61  | 15  | 15  | 1612                      | 1612                       | 372                          | 372                           | ✓  |     |    |
| 61  | 30  | 30  | 62                        | 62                         | 1302                         | 1302                          | ✓  |     |    |
| 61  | 30  | 30  | 434                       | 434                        | 1984                         | 1984                          | ✓  |     |    |
| 61  | 30  | 30  | 682                       | 682                        | 3472                         | 3472                          | ✓  |     |    |
| 61  | 30  | 30  | 806                       | 806                        | 682                          | 682                           | ✓  |     |    |
| 61  | 31  | 5   | 180                       | 1116                       | 558                          | 806                           |    | ✓   |    |
| 61  | 31  | 5   | 660                       | 372                        | 434                          | 1054                          |    | ✓   |    |
| 61  | 31  | 10  | 780                       | 558                        | 1364                         | 2604                          |    | ✓   |    |
| 61  | 31  | 10  | 900                       | 186                        | 3348                         | 3658                          |    | ✓   |    |
| 61  | 31  | 15  | 1020                      | 868                        | 3286                         | 3100                          |    | ✓   |    |
| 61  | 31  | 15  | 1140                      | 1612                       | 620                          | 372                           |    | ✓   |    |
| 61  | 31  | 30  | 1380                      | 62                         | 2356                         | 1302                          |    | ✓   |    |
| 61  | 31  | 30  | 1620                      | 682                        | 3410                         | 3472                          |    | ✓   |    |



| $q$ | $k$ | $l$ | $\log_{\xi} \xi_{\kappa}$ | $\log_{\xi} \xi_{\lambda}$ | $\log_{\xi} \omega_{\kappa}$ | $\log_{\xi} \omega_{\lambda}$ | SD | SPD | MR |
|-----|-----|-----|---------------------------|----------------------------|------------------------------|-------------------------------|----|-----|----|
| 61  | 31  | 31  | 60                        | 60                         | 2170                         | 2170                          | ✓  |     |    |
| 61  | 31  | 31  | 60                        | 1020                       | 2170                         | 3286                          |    | ✓   |    |
| 61  | 31  | 31  | 180                       | 180                        | 558                          | 558                           | ✓  |     |    |
| 61  | 31  | 31  | 300                       | 300                        | 1674                         | 1674                          | ✓  |     |    |
| 61  | 31  | 31  | 300                       | 420                        | 1674                         | 248                           |    | ✓   |    |
| 61  | 31  | 31  | 420                       | 420                        | 248                          | 248                           | ✓  |     |    |
| 61  | 31  | 31  | 420                       | 1260                       | 248                          | 992                           |    | ✓   |    |
| 61  | 31  | 31  | 540                       | 540                        | 1116                         | 1116                          | ✓  |     |    |
| 61  | 31  | 31  | 540                       | 900                        | 1116                         | 3348                          |    | ✓   |    |
| 61  | 31  | 31  | 660                       | 660                        | 434                          | 434                           | ✓  |     |    |
| 61  | 31  | 31  | 780                       | 780                        | 1364                         | 1364                          | ✓  |     |    |
| 61  | 31  | 31  | 900                       | 900                        | 3348                         | 3348                          | ✓  |     |    |
| 61  | 31  | 31  | 1020                      | 1020                       | 3286                         | 3286                          | ✓  |     |    |
| 61  | 31  | 31  | 1140                      | 1140                       | 620                          | 620                           | ✓  |     |    |
| 61  | 31  | 31  | 1260                      | 1260                       | 992                          | 992                           | ✓  |     |    |
| 61  | 31  | 31  | 1380                      | 1380                       | 2356                         | 2356                          | ✓  |     |    |
| 61  | 31  | 31  | 1500                      | 780                        | 868                          | 1364                          |    | ✓   |    |
| 61  | 31  | 31  | 1500                      | 1500                       | 868                          | 868                           | ✓  |     |    |
| 61  | 31  | 31  | 1620                      | 1620                       | 3410                         | 3410                          | ✓  |     |    |
| 61  | 31  | 31  | 1740                      | 1740                       | 1736                         | 1736                          | ✓  | ✓   |    |
| 61  | 31  | 61  | 1260                      |                            | 992                          |                               |    | ✓   |    |
| 61  | 61  | 61  |                           |                            |                              |                               | ✓  |     |    |
| 67  | 3   | 17  | 748                       | 1188                       | 0                            | 3536                          |    | ✓   |    |
| 67  | 11  | 11  | 204                       | 204                        | 2108                         | 2108                          | ✓  |     |    |
| 67  | 11  | 11  | 612                       | 612                        | 2992                         | 2992                          | ✓  |     |    |
| 67  | 11  | 11  | 1020                      | 1020                       | 340                          | 340                           | ✓  |     |    |
| 67  | 11  | 11  | 1020                      | 1836                       | 340                          | 2924                          |    | ✓   |    |
| 67  | 11  | 11  | 1428                      | 1428                       | 612                          | 612                           | ✓  |     |    |
| 67  | 11  | 11  | 1836                      | 1836                       | 2924                         | 2924                          | ✓  |     |    |
| 67  | 11  | 17  | 612                       | 132                        | 2992                         | 4420                          |    | ✓   |    |
| 67  | 11  | 17  | 1428                      | 396                        | 612                          | 1564                          |    | ✓   |    |
| 67  | 11  | 33  | 204                       | 476                        | 2108                         | 1020                          |    | ✓   |    |
| 67  | 11  | 34  | 1836                      | 594                        | 2924                         | 3128                          |    | ✓   |    |
| 67  | 17  | 17  | 132                       | 132                        | 4420                         | 4420                          | ✓  |     |    |
| 67  | 17  | 17  | 396                       | 396                        | 1564                         | 1564                          | ✓  |     |    |
| 67  | 17  | 17  | 660                       | 660                        | 136                          | 136                           | ✓  |     |    |
| 67  | 17  | 17  | 924                       | 924                        | 3876                         | 3876                          | ✓  |     |    |
| 67  | 17  | 17  | 1188                      | 1188                       | 3536                         | 3536                          | ✓  |     |    |
| 67  | 17  | 17  | 1452                      | 1452                       | 1156                         | 1156                          | ✓  |     |    |
| 67  | 17  | 17  | 1716                      | 1716                       | 1836                         | 1836                          | ✓  |     |    |
| 67  | 17  | 17  | 1980                      | 1980                       | 1428                         | 1428                          | ✓  |     |    |
| 67  | 33  | 11  | 884                       | 612                        | 2448                         | 2992                          |    | ✓   |    |
| 67  | 33  | 11  | 1156                      | 1020                       | 1088                         | 340                           |    | ✓   |    |
| 67  | 33  | 11  | 1972                      | 204                        | 3740                         | 2108                          |    | ✓   |    |
| 67  | 33  | 17  | 68                        | 1980                       | 952                          | 1428                          |    | ✓   |    |
| 67  | 33  | 17  | 340                       | 924                        | 816                          | 3876                          |    | ✓   |    |
| 67  | 33  | 17  | 2108                      | 660                        | 1972                         | 136                           |    | ✓   |    |

| $q$ | $k$ | $l$ | $\log_{\xi} \xi_{\kappa}$ | $\log_{\xi} \xi_{\lambda}$ | $\log_{\xi} \omega_{\kappa}$ | $\log_{\xi} \omega_{\lambda}$ | SD | SPD | MR |
|-----|-----|-----|---------------------------|----------------------------|------------------------------|-------------------------------|----|-----|----|
| 67  | 33  | 33  | 68                        | 68                         | 952                          | 952                           | ✓  |     |    |
| 67  | 33  | 33  | 340                       | 340                        | 816                          | 816                           | ✓  |     |    |
| 67  | 33  | 33  | 476                       | 68                         | 1020                         | 952                           |    | ✓   |    |
| 67  | 33  | 33  | 476                       | 476                        | 1020                         | 1020                          | ✓  |     |    |
| 67  | 33  | 33  | 884                       | 884                        | 2448                         | 2448                          | ✓  |     |    |
| 67  | 33  | 33  | 1156                      | 1156                       | 1088                         | 1088                          | ✓  |     |    |
| 67  | 33  | 33  | 1292                      | 1292                       | 4148                         | 4148                          | ✓  |     |    |
| 67  | 33  | 33  | 1292                      | 2108                       | 4148                         | 1972                          |    | ✓   |    |
| 67  | 33  | 33  | 1564                      | 884                        | 544                          | 2448                          |    | ✓   |    |
| 67  | 33  | 33  | 1564                      | 1564                       | 544                          | 544                           | ✓  |     |    |
| 67  | 33  | 33  | 1700                      | 1700                       | 1224                         | 1224                          | ✓  |     |    |
| 67  | 33  | 33  | 1972                      | 1972                       | 3740                         | 3740                          | ✓  |     |    |
| 67  | 33  | 33  | 2108                      | 2108                       | 1972                         | 1972                          | ✓  |     |    |
| 67  | 33  | 34  | 1700                      | 330                        | 1224                         | 1360                          |    | ✓   |    |
| 67  | 34  | 34  | 66                        | 66                         | 2720                         | 2720                          | ✓  |     |    |
| 67  | 34  | 34  | 198                       | 198                        | 408                          | 408                           | ✓  |     |    |
| 67  | 34  | 34  | 330                       | 330                        | 1360                         | 1360                          | ✓  |     |    |
| 67  | 34  | 34  | 462                       | 462                        | 272                          | 272                           | ✓  |     |    |
| 67  | 34  | 34  | 594                       | 594                        | 3128                         | 3128                          | ✓  |     |    |
| 67  | 34  | 34  | 726                       | 726                        | 4284                         | 4284                          | ✓  |     |    |
| 67  | 34  | 34  | 858                       | 858                        | 3944                         | 3944                          | ✓  |     |    |
| 67  | 34  | 34  | 990                       | 990                        | 4012                         | 4012                          | ✓  |     |    |
| 67  | 67  | 67  |                           |                            |                              |                               | ✓  |     |    |
| 71  | 3   | 36  | 840                       | 490                        | 0                            | 720                           |    | ✓   |    |
| 71  | 5   | 5   | 504                       | 504                        | 3744                         | 3744                          | ✓  |     |    |
| 71  | 5   | 5   | 1512                      | 1512                       | 3816                         | 3816                          | ✓  |     |    |
| 71  | 6   | 6   | 420                       | 420                        | 3456                         | 3456                          | ✓  |     |    |
| 71  | 6   | 35  | 420                       | 1944                       | 3456                         | 4824                          |    | ✓   | ✓  |
| 71  | 7   | 7   | 360                       | 360                        | 1152                         | 1152                          | ✓  |     |    |
| 71  | 7   | 7   | 1080                      | 1080                       | 3024                         | 3024                          | ✓  |     |    |
| 71  | 7   | 7   | 1800                      | 1800                       | 3384                         | 3384                          | ✓  |     |    |
| 71  | 9   | 7   | 1960                      | 1800                       | 1728                         | 3384                          |    | ✓   |    |
| 71  | 9   | 9   | 280                       | 280                        | 4032                         | 4032                          | ✓  |     |    |
| 71  | 9   | 9   | 1400                      | 1400                       | 4320                         | 4320                          | ✓  |     |    |
| 71  | 9   | 9   | 1960                      | 1960                       | 1728                         | 1728                          | ✓  |     |    |
| 71  | 9   | 35  | 280                       | 72                         | 4032                         | 4392                          |    | ✓   |    |
| 71  | 9   | 35  | 1400                      | 2376                       | 4320                         | 2592                          |    | ✓   |    |
| 71  | 12  | 12  | 210                       | 210                        | 2880                         | 2880                          | ✓  |     |    |
| 71  | 12  | 12  | 1050                      | 1050                       | 2160                         | 2160                          | ✓  |     |    |
| 71  | 12  | 35  | 1050                      | 1656                       | 2160                         | 144                           |    | ✓   | ✓  |
| 71  | 12  | 36  | 210                       | 1190                       | 2880                         | 1944                          |    | ✓   | ✓  |
| 71  | 18  | 5   | 980                       | 1512                       | 2088                         | 3816                          |    | ✓   | ✓  |
| 71  | 18  | 9   | 700                       | 280                        | 1080                         | 4032                          |    | ✓   | ✓  |
| 71  | 18  | 18  | 140                       | 140                        | 288                          | 288                           | ✓  |     |    |
| 71  | 18  | 18  | 700                       | 700                        | 1080                         | 1080                          | ✓  |     |    |
| 71  | 18  | 18  | 980                       | 980                        | 2088                         | 2088                          | ✓  |     |    |
| 71  | 18  | 35  | 140                       | 2088                       | 288                          | 4104                          |    | ✓   | ✓  |

| $q$ | $k$ | $l$ | $\log_{\xi} \xi_{\kappa}$ | $\log_{\xi} \xi_{\lambda}$ | $\log_{\xi} \omega_{\kappa}$ | $\log_{\xi} \omega_{\lambda}$ | SD | SPD | MR |
|-----|-----|-----|---------------------------|----------------------------|------------------------------|-------------------------------|----|-----|----|
| 71  | 35  | 35  | 72                        | 72                         | 4392                         | 4392                          | ✓  |     |    |
| 71  | 35  | 35  | 216                       | 216                        | 1656                         | 1656                          | ✓  |     |    |
| 71  | 35  | 35  | 648                       | 648                        | 3096                         | 3096                          | ✓  |     |    |
| 71  | 35  | 35  | 792                       | 792                        | 3888                         | 3888                          | ✓  |     |    |
| 71  | 35  | 35  | 936                       | 936                        | 4968                         | 4968                          | ✓  |     |    |
| 71  | 35  | 35  | 1224                      | 1224                       | 1008                         | 1008                          | ✓  |     |    |
| 71  | 35  | 35  | 1368                      | 1368                       | 1440                         | 1440                          | ✓  |     |    |
| 71  | 35  | 35  | 1656                      | 1656                       | 144                          | 144                           | ✓  |     |    |
| 71  | 35  | 35  | 1944                      | 1944                       | 4824                         | 4824                          | ✓  |     |    |
| 71  | 35  | 35  | 2088                      | 2088                       | 4104                         | 4104                          | ✓  |     |    |
| 71  | 35  | 35  | 2232                      | 2232                       | 3168                         | 3168                          | ✓  |     |    |
| 71  | 35  | 35  | 2376                      | 2376                       | 2592                         | 2592                          | ✓  |     |    |
| 71  | 36  | 7   | 770                       | 1080                       | 3312                         | 3024                          |    | ✓   | ✓  |
| 71  | 36  | 9   | 70                        | 1960                       | 4896                         | 1728                          |    | ✓   | ✓  |
| 71  | 36  | 9   | 910                       | 1400                       | 4752                         | 4320                          |    | ✓   | ✓  |
| 71  | 36  | 12  | 1190                      | 1050                       | 1944                         | 2160                          |    | ✓   | ✓  |
| 71  | 36  | 35  | 490                       | 648                        | 720                          | 3096                          |    | ✓   | ✓  |
| 71  | 36  | 36  | 70                        | 70                         | 4896                         | 4896                          | ✓  |     |    |
| 71  | 36  | 36  | 350                       | 350                        | 4536                         | 4536                          | ✓  | ✓   | ✓  |
| 71  | 36  | 36  | 490                       | 490                        | 720                          | 720                           | ✓  |     |    |
| 71  | 36  | 36  | 770                       | 770                        | 3312                         | 3312                          | ✓  |     |    |
| 71  | 36  | 36  | 910                       | 910                        | 4752                         | 4752                          | ✓  |     |    |
| 71  | 36  | 36  | 1190                      | 1190                       | 1944                         | 1944                          | ✓  |     |    |
| 71  | 71  | 71  |                           |                            |                              |                               | ✓  |     |    |
| 73  | 3   | 37  | 888                       | 72                         | 0                            | 2590                          |    | ✓   |    |
| 73  | 6   | 6   | 444                       | 444                        | 222                          | 222                           | ✓  |     |    |
| 73  | 6   | 37  | 444                       | 1080                       | 222                          | 5032                          |    | ✓   | ✓  |
| 73  | 9   | 9   | 296                       | 296                        | 148                          | 148                           | ✓  |     |    |
| 73  | 9   | 9   | 1480                      | 1480                       | 3034                         | 3034                          | ✓  | ✓   |    |
| 73  | 9   | 9   | 2072                      | 2072                       | 2146                         | 2146                          | ✓  |     |    |
| 73  | 9   | 36  | 2072                      | 814                        | 2146                         | 3552                          |    | ✓   |    |
| 73  | 9   | 37  | 296                       | 792                        | 148                          | 740                           |    | ✓   |    |
| 73  | 12  | 12  | 222                       | 222                        | 962                          | 962                           | ✓  |     |    |
| 73  | 12  | 12  | 1110                      | 1110                       | 4366                         | 4366                          | ✓  |     |    |
| 73  | 12  | 18  | 1110                      | 148                        | 4366                         | 3330                          |    | ✓   | ✓  |
| 73  | 12  | 37  | 222                       | 360                        | 962                          | 4070                          |    | ✓   | ✓  |
| 73  | 18  | 18  | 148                       | 148                        | 3330                         | 3330                          | ✓  |     |    |
| 73  | 18  | 18  | 740                       | 740                        | 3848                         | 3848                          | ✓  |     |    |
| 73  | 18  | 18  | 1036                      | 1036                       | 3700                         | 3700                          | ✓  |     |    |
| 73  | 18  | 37  | 148                       | 936                        | 3330                         | 74                            |    | ✓   | ✓  |
| 73  | 18  | 37  | 740                       | 2088                       | 3848                         | 1850                          |    | ✓   | ✓  |
| 73  | 18  | 37  | 1036                      | 504                        | 3700                         | 5180                          |    | ✓   | ✓  |
| 73  | 36  | 6   | 370                       | 444                        | 1628                         | 222                           |    | ✓   | ✓  |
| 73  | 36  | 36  | 74                        | 74                         | 4884                         | 4884                          | ✓  |     |    |
| 73  | 36  | 36  | 74                        | 962                        | 4884                         | 3182                          |    | ✓   | ✓  |
| 73  | 36  | 36  | 370                       | 370                        | 1628                         | 1628                          | ✓  |     |    |
| 73  | 36  | 36  | 518                       | 518                        | 1924                         | 1924                          | ✓  |     |    |

| $q$ | $k$ | $l$ | $\log_{\xi} \xi_{\kappa}$ | $\log_{\xi} \xi_{\lambda}$ | $\log_{\xi} \omega_{\kappa}$ | $\log_{\xi} \omega_{\lambda}$ | SD | SPD | MR |
|-----|-----|-----|---------------------------|----------------------------|------------------------------|-------------------------------|----|-----|----|
| 73  | 36  | 36  | 814                       | 370                        | 3552                         | 1628                          |    | ✓   | ✓  |
| 73  | 36  | 36  | 814                       | 814                        | 3552                         | 3552                          | ✓  |     |    |
| 73  | 36  | 36  | 962                       | 962                        | 3182                         | 3182                          | ✓  |     |    |
| 73  | 36  | 36  | 1258                      | 518                        | 814                          | 1924                          |    | ✓   | ✓  |
| 73  | 36  | 36  | 1258                      | 1258                       | 814                          | 814                           | ✓  |     |    |
| 73  | 36  | 37  | 962                       | 1944                       | 3182                         | 1332                          |    | ✓   | ✓  |
| 73  | 36  | 73  | 518                       |                            | 1924                         |                               |    | ✓   | ✓  |
| 73  | 37  | 37  | 72                        | 72                         | 2590                         | 2590                          | ✓  |     |    |
| 73  | 37  | 37  | 216                       | 216                        | 5106                         | 5106                          | ✓  |     |    |
| 73  | 37  | 37  | 360                       | 360                        | 4070                         | 4070                          | ✓  |     |    |
| 73  | 37  | 37  | 504                       | 504                        | 5180                         | 5180                          | ✓  |     |    |
| 73  | 37  | 37  | 648                       | 648                        | 3774                         | 3774                          | ✓  |     |    |
| 73  | 37  | 37  | 792                       | 792                        | 740                          | 740                           | ✓  |     |    |
| 73  | 37  | 37  | 936                       | 936                        | 74                           | 74                            | ✓  |     |    |
| 73  | 37  | 37  | 1080                      | 1080                       | 5032                         | 5032                          | ✓  |     |    |
| 73  | 37  | 37  | 1224                      | 1224                       | 444                          | 444                           | ✓  |     |    |
| 73  | 37  | 37  | 1368                      | 1368                       | 1998                         | 1998                          | ✓  |     |    |
| 73  | 37  | 37  | 1512                      | 1512                       | 1776                         | 1776                          | ✓  |     |    |
| 73  | 37  | 37  | 1656                      | 1656                       | 1480                         | 1480                          | ✓  |     |    |
| 73  | 37  | 37  | 1800                      | 1800                       | 4218                         | 4218                          | ✓  |     |    |
| 73  | 37  | 37  | 1944                      | 1944                       | 1332                         | 1332                          | ✓  |     |    |
| 73  | 37  | 37  | 2088                      | 2088                       | 1850                         | 1850                          | ✓  |     |    |
| 73  | 37  | 37  | 2232                      | 2232                       | 4958                         | 4958                          | ✓  |     |    |
| 73  | 37  | 37  | 2376                      | 2376                       | 1258                         | 1258                          | ✓  |     |    |
| 73  | 37  | 37  | 2520                      | 2520                       | 4736                         | 4736                          | ✓  |     |    |
| 73  | 73  | 73  |                           |                            |                              |                               | ✓  |     |    |
| 79  | 5   | 5   | 624                       | 624                        | 4000                         | 4000                          | ✓  |     |    |
| 79  | 5   | 5   | 1872                      | 1872                       | 5360                         | 5360                          | ✓  |     |    |
| 79  | 5   | 39  | 1872                      | 2800                       | 5360                         | 1520                          |    | ✓   |    |
| 79  | 5   | 40  | 624                       | 1326                       | 4000                         | 3760                          |    | ✓   |    |
| 79  | 8   | 8   | 390                       | 390                        | 5840                         | 5840                          | ✓  |     |    |
| 79  | 8   | 8   | 1170                      | 1170                       | 560                          | 560                           | ✓  |     |    |
| 79  | 8   | 13  | 390                       | 1200                       | 5840                         | 3520                          |    | ✓   | ✓  |
| 79  | 8   | 20  | 1170                      | 1092                       | 560                          | 2560                          |    | ✓   | ✓  |
| 79  | 10  | 10  | 312                       | 312                        | 4800                         | 4800                          | ✓  |     |    |
| 79  | 10  | 10  | 936                       | 936                        | 800                          | 800                           | ✓  |     |    |
| 79  | 10  | 39  | 312                       | 80                         | 4800                         | 5200                          |    | ✓   | ✓  |
| 79  | 10  | 40  | 936                       | 702                        | 800                          | 720                           |    | ✓   | ✓  |
| 79  | 13  | 13  | 240                       | 240                        | 2320                         | 2320                          | ✓  |     |    |
| 79  | 13  | 13  | 720                       | 720                        | 5120                         | 5120                          | ✓  |     |    |
| 79  | 13  | 13  | 1200                      | 1200                       | 3520                         | 3520                          | ✓  |     |    |
| 79  | 13  | 13  | 1680                      | 1680                       | 4480                         | 4480                          | ✓  |     |    |
| 79  | 13  | 13  | 2160                      | 2160                       | 3600                         | 3600                          | ✓  |     |    |
| 79  | 13  | 13  | 2640                      | 2640                       | 2800                         | 2800                          | ✓  |     |    |
| 79  | 20  | 10  | 1404                      | 936                        | 4400                         | 800                           |    | ✓   | ✓  |
| 79  | 20  | 20  | 156                       | 156                        | 4080                         | 4080                          | ✓  |     |    |
| 79  | 20  | 20  | 468                       | 468                        | 1440                         | 1440                          | ✓  |     |    |

| $q$ | $k$ | $l$ | $\log_{\xi} \xi_{\kappa}$ | $\log_{\xi} \xi_{\lambda}$ | $\log_{\xi} \omega_{\kappa}$ | $\log_{\xi} \omega_{\lambda}$ | SD | SPD | MR |
|-----|-----|-----|---------------------------|----------------------------|------------------------------|-------------------------------|----|-----|----|
| 79  | 20  | 20  | 1092                      | 1092                       | 2560                         | 2560                          | ✓  |     |    |
| 79  | 20  | 20  | 1092                      | 1404                       | 2560                         | 4400                          |    | ✓   | ✓  |
| 79  | 20  | 20  | 1404                      | 1404                       | 4400                         | 4400                          | ✓  |     |    |
| 79  | 20  | 39  | 156                       | 400                        | 4080                         | 1120                          |    | ✓   | ✓  |
| 79  | 20  | 40  | 468                       | 1014                       | 1440                         | 2400                          |    | ✓   | ✓  |
| 79  | 39  | 39  | 80                        | 80                         | 5200                         | 5200                          | ✓  |     |    |
| 79  | 39  | 39  | 400                       | 400                        | 1120                         | 1120                          | ✓  |     |    |
| 79  | 39  | 39  | 560                       | 560                        | 2960                         | 2960                          | ✓  |     |    |
| 79  | 39  | 39  | 880                       | 880                        | 2480                         | 2480                          | ✓  |     |    |
| 79  | 39  | 39  | 1360                      | 1360                       | 3200                         | 3200                          | ✓  |     |    |
| 79  | 39  | 39  | 1520                      | 1520                       | 4960                         | 4960                          | ✓  |     |    |
| 79  | 39  | 39  | 1840                      | 1840                       | 1200                         | 1200                          | ✓  |     |    |
| 79  | 39  | 39  | 2000                      | 2000                       | 6000                         | 6000                          | ✓  |     |    |
| 79  | 39  | 39  | 2320                      | 2320                       | 1600                         | 1600                          | ✓  |     |    |
| 79  | 39  | 39  | 2480                      | 2480                       | 4160                         | 4160                          | ✓  |     |    |
| 79  | 39  | 39  | 2800                      | 2800                       | 1520                         | 1520                          | ✓  |     |    |
| 79  | 39  | 39  | 2960                      | 2960                       | 3040                         | 3040                          | ✓  |     |    |
| 79  | 40  | 5   | 546                       | 1872                       | 5280                         | 5360                          |    | ✓   | ✓  |
| 79  | 40  | 8   | 858                       | 1170                       | 3360                         | 560                           |    | ✓   | ✓  |
| 79  | 40  | 13  | 234                       | 2160                       | 5040                         | 3600                          |    | ✓   | ✓  |
| 79  | 40  | 13  | 1014                      | 720                        | 2400                         | 5120                          |    | ✓   | ✓  |
| 79  | 40  | 39  | 78                        | 880                        | 1760                         | 2480                          |    | ✓   | ✓  |
| 79  | 40  | 39  | 702                       | 1360                       | 720                          | 3200                          |    | ✓   | ✓  |
| 79  | 40  | 39  | 1482                      | 2320                       | 2640                         | 1600                          |    | ✓   | ✓  |
| 79  | 40  | 40  | 78                        | 78                         | 1760                         | 1760                          | ✓  |     |    |
| 79  | 40  | 40  | 234                       | 234                        | 5040                         | 5040                          | ✓  |     |    |
| 79  | 40  | 40  | 546                       | 546                        | 5280                         | 5280                          | ✓  |     |    |
| 79  | 40  | 40  | 702                       | 702                        | 720                          | 720                           | ✓  |     |    |
| 79  | 40  | 40  | 858                       | 858                        | 3360                         | 3360                          | ✓  |     |    |
| 79  | 40  | 40  | 1014                      | 1014                       | 2400                         | 2400                          | ✓  |     |    |
| 79  | 40  | 40  | 1326                      | 78                         | 3760                         | 1760                          |    | ✓   | ✓  |
| 79  | 40  | 40  | 1326                      | 1326                       | 3760                         | 3760                          | ✓  |     |    |
| 79  | 40  | 40  | 1482                      | 1482                       | 2640                         | 2640                          | ✓  |     |    |
| 79  | 79  | 79  |                           |                            |                              |                               | ✓  |     |    |
| 81  | 4   | 41  | 820                       | 1040                       | 4920                         | 2214                          |    | ✓   |    |
| 81  | 5   | 41  | 656                       | 400                        | 2460                         | 164                           |    | ✓   |    |
| 81  | 5   | 41  | 656                       | 1680                       | 2460                         | 5248                          |    | ✓   |    |
| 81  | 8   | 40  | 410                       | 574                        | 1230                         | 5576                          |    | ✓   |    |
| 81  | 8   | 41  | 410                       | 80                         | 1230                         | 6068                          |    | ✓   |    |
| 81  | 10  | 40  | 328                       | 82                         | 2050                         | 4674                          |    | ✓   |    |
| 81  | 10  | 41  | 328                       | 2480                       | 2050                         | 2542                          |    | ✓   |    |
| 81  | 20  | 20  | 164                       | 164                        | 5658                         | 5658                          | ✓  |     |    |
| 81  | 20  | 41  | 164                       | 3120                       | 5658                         | 82                            |    | ✓   | ✓  |
| 81  | 40  | 40  | 82                        | 82                         | 4674                         | 4674                          | ✓  |     |    |
| 81  | 40  | 40  | 82                        | 738                        | 4674                         | 2706                          | ✓  |     |    |
| 81  | 40  | 40  | 574                       | 574                        | 5576                         | 5576                          | ✓  |     |    |
| 81  | 40  | 40  | 574                       | 1394                       | 5576                         | 4264                          | ✓  |     |    |

| $q$ | $k$ | $l$ | $\log_{\xi} \xi_{\kappa}$ | $\log_{\xi} \xi_{\lambda}$ | $\log_{\xi} \omega_{\kappa}$ | $\log_{\xi} \omega_{\lambda}$ | SD | SPD | MR |
|-----|-----|-----|---------------------------|----------------------------|------------------------------|-------------------------------|----|-----|----|
| 81  | 40  | 41  | 82                        | 1680                       | 4674                         | 5248                          |    | ✓   | ✓  |
| 81  | 40  | 41  | 574                       | 2640                       | 5576                         | 3198                          |    | ✓   | ✓  |
| 81  | 41  | 41  | 80                        | 80                         | 6068                         | 6068                          | ✓  |     |    |
| 81  | 41  | 41  | 80                        | 720                        | 6068                         | 2132                          | ✓  |     |    |
| 81  | 41  | 41  | 400                       | 400                        | 164                          | 164                           | ✓  |     |    |
| 81  | 41  | 41  | 400                       | 2960                       | 164                          | 1476                          | ✓  |     |    |
| 81  | 41  | 41  | 560                       | 560                        | 3936                         | 3936                          | ✓  |     |    |
| 81  | 41  | 41  | 560                       | 1520                       | 3936                         | 2624                          | ✓  |     |    |
| 81  | 41  | 41  | 880                       | 880                        | 1066                         | 1066                          | ✓  |     |    |
| 81  | 41  | 41  | 880                       | 1360                       | 1066                         | 3034                          | ✓  |     |    |
| 81  | 41  | 41  | 1040                      | 1040                       | 2214                         | 2214                          | ✓  |     |    |
| 81  | 41  | 41  | 1040                      | 2800                       | 2214                         | 246                           | ✓  |     |    |

| $q$ | Maps | None | SD only | SP only | SD+SP | SP+MR | SD+SP+MR |
|-----|------|------|---------|---------|-------|-------|----------|
| 5   | 1    | 0    | 1       | 0       | 0     | 0     | 0        |
| 7   | 5    | 4    | 1       | 0       | 0     | 0     | 0        |
| 9   | 3    | 2    | 1       | 0       | 0     | 0     | 0        |
| 11  | 16   | 11   | 3       | 1       | 1     | 0     | 0        |
| 13  | 33   | 26   | 4       | 2       | 1     | 0     | 0        |
| 17  | 58   | 50   | 6       | 0       | 0     | 2     | 0        |
| 19  | 70   | 58   | 8       | 4       | 0     | 0     | 0        |
| 23  | 113  | 101  | 8       | 1       | 0     | 2     | 1        |
| 25  | 63   | 52   | 7       | 3       | 0     | 1     | 0        |
| 27  | 54   | 48   | 4       | 2       | 0     | 0     | 0        |
| 29  | 183  | 163  | 13      | 7       | 0     | 0     | 0        |
| 31  | 209  | 190  | 13      | 0       | 0     | 6     | 0        |
| 37  | 315  | 290  | 16      | 8       | 1     | 0     | 0        |
| 41  | 382  | 356  | 18      | 2       | 0     | 6     | 0        |
| 43  | 430  | 400  | 20      | 10      | 0     | 0     | 0        |
| 47  | 515  | 485  | 20      | 1       | 0     | 8     | 1        |
| 49  | 264  | 238  | 16      | 7       | 0     | 3     | 0        |
| 53  | 663  | 625  | 25      | 13      | 0     | 0     | 0        |
| 59  | 820  | 779  | 27      | 13      | 1     | 0     | 0        |
| 61  | 879  | 836  | 28      | 14      | 1     | 0     | 0        |
| 67  | 1072 | 1024 | 32      | 16      | 0     | 0     | 0        |
| 71  | 1199 | 1151 | 32      | 4       | 0     | 11    | 1        |
| 73  | 1276 | 1227 | 33      | 3       | 1     | 12    | 0        |
| 79  | 1493 | 1438 | 37      | 2       | 0     | 16    | 0        |
| 81  | 381  | 356  | 15      | 7       | 0     | 3     | 0        |

TABLE 2. External symmetries of regular maps on  $PSL(2, q)$

## REFERENCES

- [1] The GAP Group, Groups, Algorithms, and Programming, Version 4.9.1, May 2018, <https://www.gap-system.org>.
